# Supplementary material for: FEDEX: An Explainability Framework for Data Exploration Steps
Source: arXiv:2209.06260 source file (2022-09-13)
Supplement: Supplementary file 1 [file revision_appendix.tex]

\section*{Appendix - Additional Experiments}
% We provide additional experimental results asked by the reviewers. These complement our existing experimental results and will be included in the full version of the paper. 

\begin{figure}[h]
    \centering 
    \includegraphics[scale=0.35]{images/Baselines NL Explanations/NL baselines.png}
    \caption{\ag{R1D9:}\reva{User study results for baselines augmented with NL explanations}}
    \label{fig:NL_baseline_userstudy}
\end{figure}

\reva{
\paratitle{Qualitative comparison to custom hybrid baselines}
We have augmented the \seedb\ and \rath\ baselines with textual explanations (in addition to their `organic' visualizations) and performed an additional user study.
The study included 4 participants that considered the Credit Card Customers dataset and its notebook from the first user study with the five relevant queries in Table \ref{tbl:queries}. We have asked an expert to add a textual description to each baseline visualization included in a notebook and presented them to the participants. 
The results appear in Figure \ref{fig:NL_baseline_userstudy} and indicate that even with textual explanations for the baselines, \sys\ is able to generate explanations that are significantly more coherent, insightful, and useful. In particular, the scores were $5.52$ for \sys, $3.17$ for \seedb\ augmented with textual explanations, and $3.42$ for \rath\ augmented with textual explanations. 
}

% \begin{figure}[h]
%     \centering 
%     \includegraphics[width=2.6in]{images/Baselines NL Explanations/NL baselines.png}
%     \caption{User Study with NL explanations for baselines}
%     \label{fig:NL_baseline_userstudy}
% \end{figure}
